# Supplementary material for: SAMCIRT: A Simultaneous Reconstruction and Affine Motion Compensation Technique for Four Dimensional Computed Tomography (4DCT)
Source: arXiv:2402.04480 source file (2025-10-07)
Supplement: Supplementary file 1 [file Appendix.tex]

\section*{Data availability}
Data can be made available upon request.

\section*{Appendix: determination of feasible subscans}
Although the method has been empirically validated on both simulated and real projection datasets, the choice for the best subscans still remains an open question. This section does not give an exact solution to the problem but provides an insight in choosing such subscans so that the method works with an improved performance.

The trivial fact is that the choice of feasible subscans strongly depend on the data. In theory, one needs to determine at which projection there is more motion than the previous \cite{Ens10}. More specifically, if the subscans are of an equal size, the method performs well in estimating monotone motions. However, if the motion is more complicated (e.g., natural breathing), continuous motion estimation must be considered. 

Because the object is assumed to be static in each subscan, there should be no significant differences between the metric values of the pairs of two successive projections within. For instance, it can be seen from the \cref{fig:SSIMs_scaffold} that there are five points dropped in the SSIM values, which results in six subscans that are chosen for validating the scaling estimation on the bone scaffold's real projection dataset.

In order to study the problem in a general case, let us consider a dynamic full scan consists of $N+1$ projections $\bm{y}_1, \bm{y}_2, \hdots, \bm{y}_{N+1}$. 

\begin{definition}[feasible subscan]
A subscan is said to be feasible if there is not a significant change of the object through the projections within it. In other words, the pairs of two adjacent projections within it are relatively approximated in any specific metric.
\end{definition}

The problem \textit{feasible subscan partition} of projections can be mathematically formulated using the SSIM metric as the following:

\begin{problem}[feasible subscan partition]\label{prob:subscan}
Let $\bm{s} = \left[s_1, s_2, \hdots, s_N \right]^T \in \left[0, 1 \right]^{N}$ be a vector that collects the SSIM values of all pairs of two adjacent projections. More specifically,
\begin{equation}
    s_i = \text{SSIM}\left( \bm{y}_i, \bm{y}_{i+1} \right), \forall  i=\overline{1, {N}}.
\end{equation}

One needs to partition the finite set $\mathcal{S} = \left \{1, 2, 3, \hdots, N\right \}$ into $n$ mutually exclusive subsets $\mathcal{S}_1, \mathcal{S}_2, \hdots \text{and } \mathcal{S}_n$, in which each contains consecutive integers so that the projections corresponding to the same subset of indices are similar under SSIM standard. Mathematically speaking, for any integer $k$ such that $1 \le k \le n$, the following inequality holds for a given specific value $\epsilon$:
\begin{equation}
    \left | s_i - s_j \right | < \epsilon, \hspace{0.15cm} \forall i, j \in \mathcal{S}_k.
\end{equation}

On the other hand, in order to reduce the complexity of the computation \cref{obj_sum}, the optimal value of the number of feasible subscans must be minimized. As a result, it yields the following statistical integer programming problem:
\begin{equation}
    \left [\widehat{n}, \widehat{\sigma}_1, \hdots, \widehat{\sigma}_{\widehat{n}} \right] = \argmin_{n, \sigma_1, \hdots, \sigma_{n}} g\left(n, \sigma_1, \hdots, \sigma_n \right),
\end{equation}
with 
\begin{equation}\label{eq:g}
    g\left(n, \sigma_1, \hdots, \sigma_n \right) = n + \lambda \sum_{k=1}^{n} \sigma_k^2,
\end{equation}
where $\sigma_k^2 = Var\left(\left\{s_l | l \in \mathcal{S}_k \right \} \right) \in [0, 1]$, and $\lambda > 0$ is the trade-off coefficient between the integer term and the statistical term.
\end{problem}

\begin{theorem}Solution(s) to the problem ``feasible subscan partition'' exist only when the trade-off coefficient $\lambda > 1$.
\end{theorem}

\begin{proof}
Let us consider the contradictory assumption $\lambda \le 1$. Assume that the projections are partitioned into $\widehat{n} \ge 2$ feasible subscans. Evidently, the variance of the SSIM values satisfies $0 \lesssim \widehat{\sigma}_i^2 \le 1$ $\forall i=\overline{1, \widehat{n}}$ due to the boundedness of the chosen metric. As a result, if $ \widehat{n} \ge 2$ then it yields:
\begin{equation}
    g\left(\widehat{n}, \widehat{\sigma}_1, \hdots, \widehat{\sigma}_n \right) = \widehat{n} + \lambda \sum_{k=1}^{n} \widehat{\sigma}_k^2 \ge 2 \ge 1 + \lambda \widehat{\sigma}^2,
\end{equation}
which is the value of the objective function if and only if there is the subscan identical to the full scan, i.e., $\widehat{n} \equiv 1$ and $\widehat{\sigma}^2 \equiv Var\left( \left\{s_i | i \in \mathcal{S} \right\} \right)$. This contradiction demonstrates the negation of the contradictory assumption.
\end{proof}
